# Supplementary material for: Assessing the Reliability of Truncated Coupled Cluster Wavefunction: Estimating the Distance from the Exact Solution
Source: arXiv:2508.15681 ancillary file (2025-08-21)
Supplement: Supplementary file 1 [file Supporting_Information.pdf]

# Supporting Information for "Assessing the Reliability of Truncated Coupled Cluster Wavefunction: Estimating the Distance from the Exact Solution"

Ádám Ganyecz,*,† Zsolt Benedek,‡,¶ Klára Petrov,§ Gergely Barcza,† András Olasz,†,‖ Miklós A. Werner,† and Örs Legeza†,⊥,#

†*Strongly Correlated Systems "Lendület" Research Group, Wigner Research Centre for Physics, H-1525, Budapest, Hungary*

‡*Department of Physics of Complex Systems, Eötvös Loránd University, Egyetem tér 1-3, H-1053 Budapest, Hungary*

¶*MTA–ELTE Lendület "Momentum" NewQubit Research Group, Pázmány Péter, Sétány 1/A, 1117 Budapest, Hungary*

§*Department of Physical Chemistry and Materials Science, Faculty of Chemical Technology and Biotechnology, Budapest University of Technology and Economics, Műegyetem rkp. 3., H-1111 Budapest, Hungary*

‖*Furukawa Electric Institute of Technology Ltd., Késmárk street 28/A, H-1158 Budapest, Hungary*

⊥ *Institute for Advanced Study,Technical University of Munich, Lichtenbergstrasse 2a, 85748 Garching, Germany*

#*Parmenides Stiftung, Hindenburgstr. 15, 82343, Pöcking, Germany*

E-mail: ganyecz.adam@wigner.hun-ren.hu

Contents of Supporting Information:

- List of all studied species in Table S1., and geometries in geometries.zip.
- Validation of the introduced approximations (Section S1)
- $\tilde{d}$ values for W4-17 (Sheet S1) and transition metal species (Sheet S6)
- other MR diagnostics for W4-17 species (Sheet S2)
- Pearson, Spearman, Kendall correlation statistics (Sheet S3-S5, Table S3-S4.)
- Comparison of $\tilde{d}$-s for alkanes and halogenated alkanes (Table S5.)

Table S1: List of all studied species. For TM species the used state is also presented, if the used state differs from what is listed in the source then state in the reference is also shown in parantheses.

| **W4-17 (SR)** Ref. 1 | | | | | |
|---|---|---|---|---|---|
| Acetaldehyde | $C_2F_6$ | $CH_4$ | Formic acid | HS | Propane |
| Acetic acid | $C_2H_2$ | $CHF_3$ | Formic-anhydride | Ketene | Propene |
| AlCl | $C_2H_3F$ | cis-$C_2F_2Cl_2$ | Furan | Methanol | Propyne |
| $AlCl_3$ | $C_2H_4$ | $Cl_2$ | Glyoxal | n-butane | Pyrrole |
| AlF | $C_2H_5F$ | ClCN | $H_2CCN$ | n-pentane | $S_2$ |
| $AlF_3$ | $C_2H_6$ | ClCOF | $H_2CN$ | $N_2$ | $S_2O$ |
| AlH | CCH | ClF | $H_2CO$ | $N_2H$ | $SF_6$ |
| $AlH_3$ | $CCl_2$ | ClNO | $H_2NO$ | $N_2H_4$ | $Si_2H_6$ |
| Allene | $CCl_2H_2$ | ClO | $H_2O$ | $N_2O$ | SiF |
| Allyl | $CCl_2O$ | CN | $H_2S$ | $N_2O_4$ | $SiF_4$ |
| $B_2H_6$ | $CCl_3H$ | CO | HCCF | NCCN | SiH |
| Benzene | $CCl_4$ | $CO_2$ | HCl | NH | $SiH_3F$ |
| Beta-lactim | $CClH_3$ | CS | $HClO_4$ | $NH_2$ | $SiH_4$ |
| BF | CF | $CS_2$ | HCN | $NH_2Cl$ | Silole |
| $BF_3$ | $CF_2$ | Cyclobutadiene | HCNH | $NH_2F$ | SiO |
| BH | $CF_2Cl_2$ | Cyclobutane | HCNO | $NH_2OH$ | SO |
| $BH_3$ | $CF_4$ | Cyclobutene | HCO | $NH_3$ | $SO_2$ |
| $BHF_2$ | CH | Cyclopentadiene | HCOF | NO | $SO_3$ |
| BN $^3\Pi$ | $CH_2$ $^1A_1$ | Cyclopropane | HF | $NO_2$ | SSH |
| Borole | $CH_2$ $^3B_1$ | Cyclopropene | HNC | $O_2$ | trans-butadiene |
| cis-HCOH | $CH_2C$ | Cyclopropyl | HNCO | OCS | trans-HCOH |
| cis-HONO | $CH_2CH$ | Dioxetan-2-one | HNNN | OH | trans-HONO |
| cis-HOOO | $CH_2ClF$ | Dioxetane | HNO | Oxadiazole | trans-HOOO |
| cis-$N_2H_2$ | $CH_2F_2$ | Dioxirane | HOCl | Oxetane | trans-$N_2H_2$ |
| $C_2Cl_2$ | $CH_2NH$ | Dithiotane | HOClO | Oxirane | Tetrahedrane |
| $C_2Cl_4$ | $CH_2NH_2$ | Ethanol | $HOClO_2$ | Oxirene | Thiophene |
| $C_2Cl_6$ | $CH_3$ | $F_2$ | HOCN | $P_2$ | trans-$C_2F_2Cl_2$ |
| $C_2ClH$ | $CH_3F$ | $F_2CO$ | HOF | $P_4$ | |
| $C_2ClH_3$ | $CH_3NH$ | FCCF | HONC | $PF_3$ | |
| $C_2ClH_5$ | $CH_3NH_2$ | FNO | HOO | $PF_5$ | |
| $C_2F_4$ | $CH_3PH_2$ | Formamide | HOOH | $PH_3$ | |

| **W4-17 (MR)** Ref. 1 | | | | | |
|---|---|---|---|---|---|
| $B_2$ | $Cl_2O$ | $ClO_3$ | $F_2O$ | $O_3$ | $S_3$ |
| BN $^1\Sigma$ | $ClF_3$ | ClOO | $FO_2$ | OClO | $S_4$ |
| $C_2$ | $ClF_5$ | ClOOCl | FOOF | OF | |

| **3d-MLBE-SR** | | **3d-MLBE-MR** Ref. 2 | | | |
|---|---|---|---|---|---|
| CrCl $^6\Sigma^+$ | ZnH $^2\Sigma^+$ | TiCl $^4\Phi$ | CrH $^6\Sigma^+$ | CoH $^3\Phi$ | ZnO $^1\Sigma$ |
| MnCl $^7\Sigma^+$ | ZnS $^1\Sigma$ | VH $^5\Delta$ | CrO $^5\Pi$ | CoCl $^5\Delta$ ($^3\Phi$) | |
| FeCl $^6\Delta$ | ZnCl $^2\Sigma$ | VO $^4\Sigma^-$ | MnS $^6\Sigma^+$ | NiCl $^2\Pi$ | |
| CuCl $^1\Sigma$ | | VCl $^5\Delta$ | FeH $^6\Delta$ ($^4\Delta$) | CuH $^1\Sigma^+$ | |

| **3d-TM-9** | | | **4d-TM-9** (all SR); Ref. 3 | | |
|---|---|---|---|---|---|
| ScB $^5\Sigma^-$ (MR) | TiB $^6\Delta$ (MR) | VB $^7\Sigma^+$ (MR) | YB $^5\Sigma^-$ | ZrB $^6\Delta$ | NbB $^5\Phi$ |
| ScC $^4\Pi$ (MR) | TiC $^3\Sigma^+$ (SR) | VC $^2\Delta$ (MR) | YC $^4\Sigma$ ($^4\Phi$) | ZrC $^3\Sigma^+$ | NbC $^2\Delta$ |
| ScS $^2\Sigma^+$ (MR) | TiS $^3\Delta$ (SR) | VS $^4\Sigma^-$ (MR) | YS $^2\Sigma^+$ | ZrS $^3\Sigma^+$ | NbS $^4\Sigma^-$ |

| **TM-MR** | | | | | |
|---|---|---|---|---|---|
| 3d species from Ref 4 | | | | | |
| $ScB_2$ $^2A_1$ | VSe $^4\Sigma^-$ | $CrO_3$ $^1A_1$ | FeS $^5\Delta$ | NiH $^2\Delta$ | NiGe $^1\Sigma^+$ |
| TiB $^6\Sigma^+$ | $VO_2$ $^2A_1$ | $CrO_2Cl$ $^2A'$ | CoO $^4\Delta$ | NiO $^3\Sigma^-$ | |
| TiSe $^3\Delta$ | CrN $^4\Sigma^-$ | MnO $^6\Sigma^+$ | CoSi $^2\Sigma^-$ | NiS $^3\Sigma^-$ | |
| VS $^4\Sigma^-$ | CrS $^5\Pi$ | FeO $^5\Delta$ | CoGe $^2\Sigma^-$ | NiSi $^1\Sigma^+$ | |
| 4d species from Ref 5 | | | | | |
| YN $^1\Sigma$ | $ZrO_2$ $^1A_1$ | $TcF_3$ $^5A_1$ | RuO $^5\Delta$ | $RuBr_3$ $^6A_1$ | RhSi $^2\Sigma$ |
| $YB_2$ $^2A_1$ | $NbO_2$ $^2A_1$ | $TcF_4$ $^4A_2$ | RuS $^5\Delta$ | RhC $^2\Sigma$ | RhGe $^2\Sigma$ |
| $YC_2$ $^2A_1$ ($^2B_2$) | $MoO_2$ $^3B_1$ | RuH $^4\Sigma$ | RuGe $^3\Delta$ | RhO $^4\Sigma$ | |
| species from Ref 6 | | | | | |
| 3d | | | | 4d | 5d |
| ScO $^2\Sigma^+$ | TiF $^4\Phi$ | FeCN $^6\Delta$ | $CuCl_2$ $^2\Pi$ | $Mo_2$ $^1\Sigma^+$ | $W_2$ $^1\Sigma^+$ |
| $Sc_2$ $^5\Sigma$ | $V_2$ $^3\Sigma$ | CoS $^4\Delta$ | | $MoO_3$ $^1A_1$ | IrO $^2\Delta$ |
| TiH $^4\Phi$ | $Cr_2$ $^1\Sigma$ | NiF $^2\Pi$ | | RuC $^1\Sigma^+$ | PtO $^3\Sigma^-$ |
| TiN $^2\Sigma^+$ | $Fe_2$ $^9\Sigma^-$ | $NiO_2$ $^3B_1$ | | $AgCl_2$ $^2\Pi$ | |

# S1 Validation of the introduced approximations

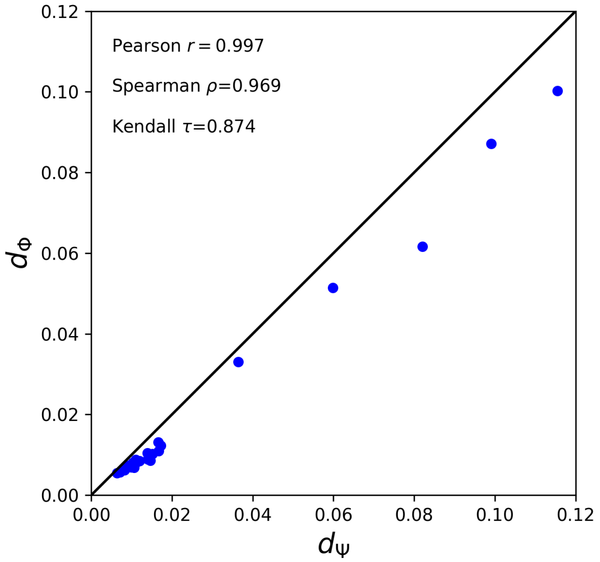


Figure S1: Comparison of $d_\Psi$ values when all coefficients considered and only up to double excitations ($d_\Phi$). Note, that BN, BN $^3\Pi$ and $C_2$ are only compared up to 7-tuple excitation, $NH_3$ and $PH_3$ up to 6-tuple excitations, respectively.

The first approximation used in this work is the truncation of the $\Psi$ wavefunction up to double excitations ($\Phi$), instead of using all the $c$ coefficients due to their large number. To justify the truncation we determined $d_\Psi$ and $d_\Phi$ values for species from W4-17 dataset, where FCI reference calculations were possible to perform (AlH, $AlH_3$, $B_2$, BH, $BH_3$, BN, BN $^3\Pi$, $C_2$, CH, $CH_2$-singlet, $CH_2$-triplet, $CH_3$, $H_2O$, $H_2S$, HCl, HF, HS, NH, $NH_2$, $NH_3$, OH, $PH_3$, SiH). In Fig. S1, $d_\Phi$ is presented as a function of $d_\Psi$. It is clear that the truncation leads to lower $d$ values, but $d_\Phi$ does not lose its descriptive power ($r = 0.997$, $\rho = 0.969$, $\tau = 0.874$).

The next approximation is the usage of DMRG instead of FCI as an FCI solver. To find the appropriate truncation error for DMRG, which handles its accuracy, we studied the effect of truncation error on $d_\gamma$ and $d_\Phi$ values and presented the error statistics compared to the FCI reference values in Table S2. From this small sample, we can see that $d$-s can even reach 0.2, but most values are below 0.1. In this case, we would like errors that are at least an order of magnitude smaller, around 0.01. DMRG with $10^{-7}$ truncation error

Table S2: Error statistics of $d_\Phi$ and $d_\gamma$ with different DMRG truncation errors using FCI results as reference.

| truncation | $d_\Phi$ | | | | $d_\gamma$ | | | |
|---|---|---|---|---|---|---|---|---|
| error | MAX | MSD | MAD | RMSD | MAX | MSD | MAD | RMSD |
| $10^{-3}$ | 0.2104 | 0.1237 | 0.1237 | 0.1284 | 0.0999 | 0.0316 | 0.0450 | 0.0488 |
| $10^{-4}$ | 0.0607 | 0.0264 | 0.0278 | 0.0324 | 0.0771 | -0.0025 | 0.0124 | 0.0202 |
| $10^{-5}$ | 0.0057 | 0.0008 | 0.0023 | 0.0029 | 0.0075 | -0.0028 | 0.0028 | 0.0032 |
| $10^{-6}$ | 0.0073 | -0.0001 | 0.0007 | 0.0016 | 0.0014 | -0.0005 | 0.0005 | 0.0006 |
| $10^{-7}$ | 0.0002 | -0.0001 | 0.0001 | 0.0001 | 0.0002 | -0.0001 | 0.0001 | 0.0001 |

provides basically the same $d$ values as the reference FCI. $10^{-6}$ and $10^{-5}$ truncation error gives acceptable error statistics with RMSDs of 0.0016 and 0.0029 for $d_\Phi$, and 0.0006 and 0.0032 for $d_\gamma$, respectively. The maximum errors are also smaller than 0.01. However, $10^{-3}$ and $10^{-4}$ truncation errors have RMSDs greater than 0.02, which is not acceptable. Considering these, at least a truncation error of $10^{-5}$ is needed for reasonable results.

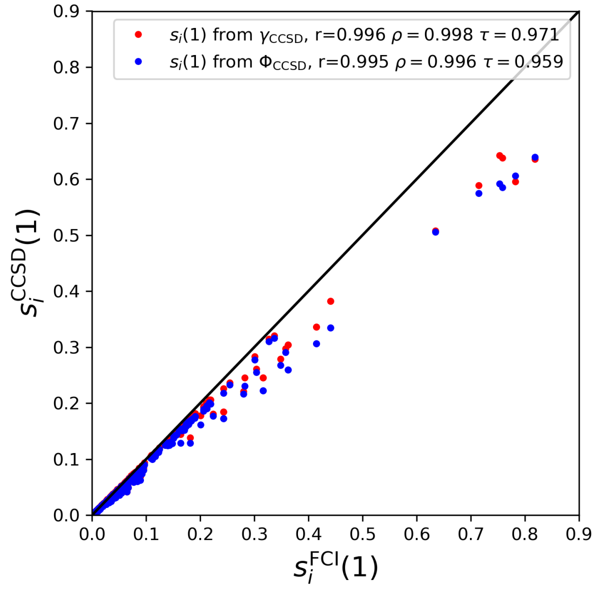


Figure S2: Entropies from CCSD calculations determined from $\gamma_{CCSD}$ and $\Phi_{CCSD}$ compared to entropies from FCI

The third approximation is the usage of a subspace instead of the whole orbital set. The orbital selection procedure is based on $s_i(1)$ values, therefore first we checked how CCSD and FCI entropies relate to each other (Fig. S2). CCSD entropies were determined from both RDM-s and $\Phi$, because this is the data available from the calculation for which $d$ has

to be determined. Generally, entropies from RDM-s of CCSD are smaller, and from $\Phi$-s are even smaller, but they are correlated, ($r > 0.99$, $\rho > 0.99$, $\tau > 0.95$).

In the following, we turn the focus to the analysis of $d$ with respect to the active space size for the three proposed workflows exemplified on the four species with considerable $d$ values ($B_2$, BN, BN $^3\Pi$, $C_2$). Due to the active space, we distinguish between $d^{\mathrm{a}}$ and $d^{\mathrm{b}}$. In Fig. S3 it can be seen that in general the quality of the active spaces ($d^{\mathrm{AS}}$) is better with more orbitals. Also, using natural orbitals increases the quality even better at first glance. $B_2$ and BN with canonical orbitals have a bump at 9 and 14 orbitals, respectively. The corresponding $d^{\mathrm{a}}$ and $d^{\mathrm{b}}$-s with smaller active spaces differ considerably from the reference values. This local maximum might indicate that not all important orbitals are included. After the local maximum in $d^{\mathrm{AS}}$, the $d^{\mathrm{a}}$ and $d^{\mathrm{b}}$ values with canonical orbitals are converging to the reference. Although NO transformation produces active spaces with lower $d^{\mathrm{AS}}$ and the corresponding $d^{\mathrm{a}}$ and $d^{\mathrm{b}}$ values have smaller difference between them, but the reference is outside of their interval, especially for $C_2$. This raises a concern that the NO-transformation might introduce a bias to the CCSD solution leading to smaller $d$ values.

In some cases $d^{\mathrm{a}}$ have faster convergence ($B_2$, $C_2$), in other cases $d^{\mathrm{b}}$ is better (BN$^3\Pi$). However, one can see that the reference value is mostly within the $[d^{\mathrm{b}}; d^{\mathrm{a}}]$ interval, regardless of the active space size. Based on this observation, we introduce their average noted as $\tilde{d}$:

$$\tilde{d}_{\Phi} = \frac{d^{\mathrm{a}}_{\Phi} + d^{\mathrm{b}}_{\Phi}}{2} \tag{1a}$$

$$\tilde{d}_{\gamma} = \frac{d^{\mathrm{a}}_{\gamma} + d^{\mathrm{b}}_{\gamma}}{2} \tag{1b}$$

$\tilde{d}$ have better convergence in most cases and will be used from now, to estimate the $d$ values in question.

However, these systems are too small, therefore we tested the convergence on a larger species with considerable $\tilde{d}$, namely $N_2O_4$ (Fig. S4).

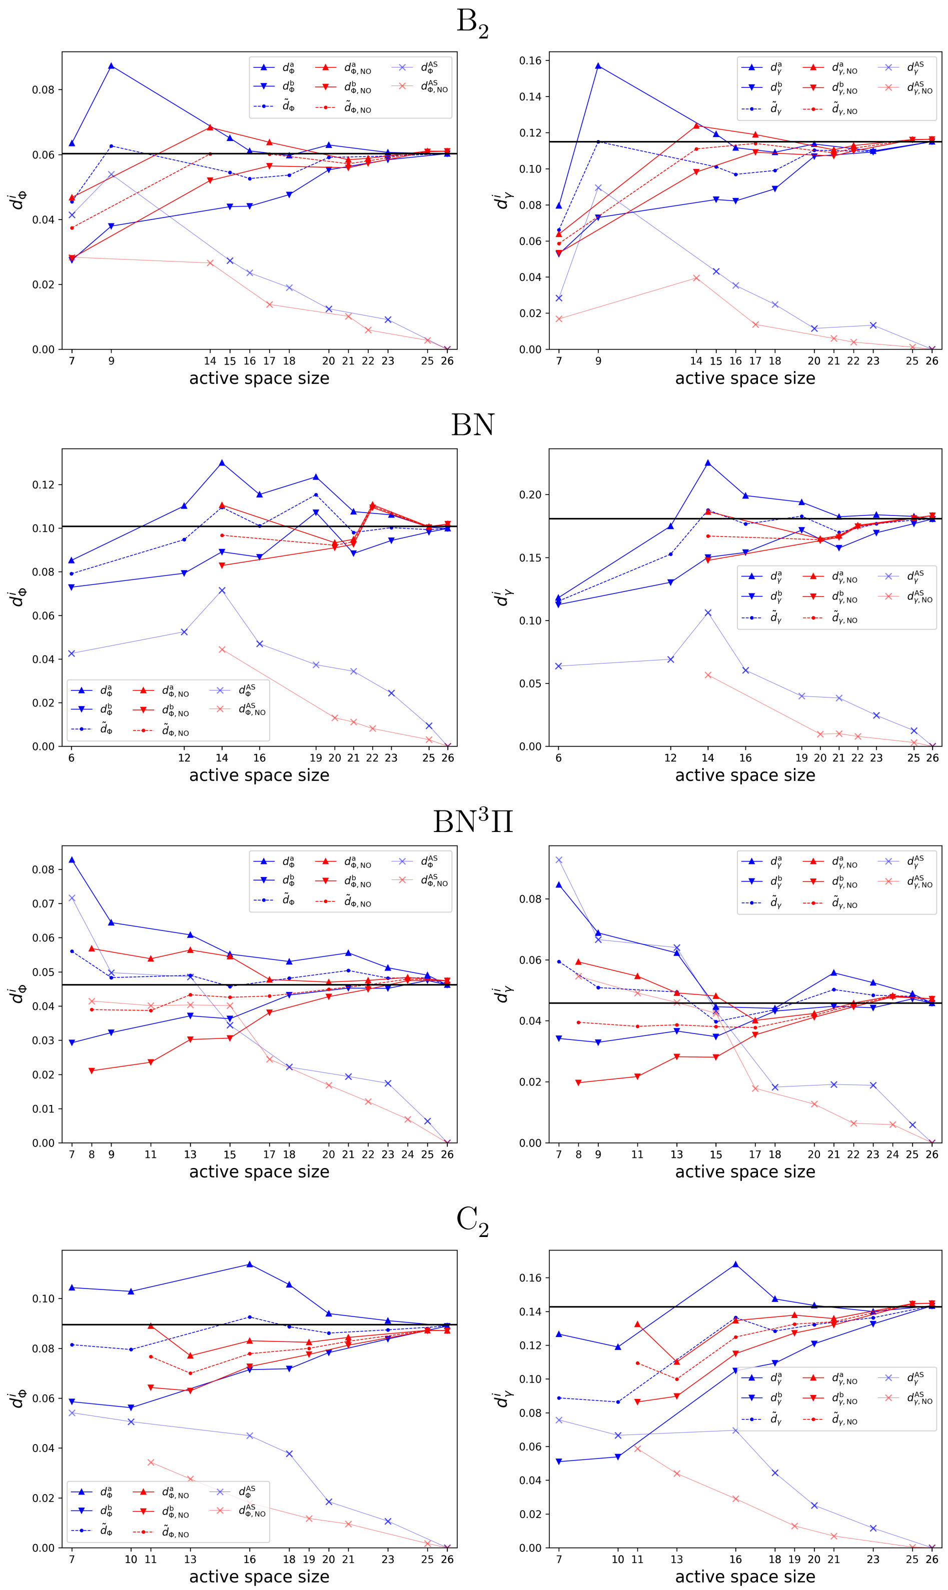


Figure S3: The dependence of $d^{\mathrm{a}}$, $d^{\mathrm{b}}$, and $\tilde{d}$ on active space size for $B_2$, BN, BN $^3\Pi$, and $C_2$. Left figures are $d_\Phi$, right figures are for $d_\gamma$ values, however $d$-s are determined for all active space selection procedure considered in this work. Upward triangles are for $d^{\mathrm{a}}$, downward triangles for $d^{\mathrm{b}}$, dots are for their average, $\tilde{d}$, and crosses are for $d^{\mathrm{AS}}$ values. Blue color represents canonical orbital selection, while red ones used natural orbitals. The black line shows the true $d_\Phi$ or $d_\gamma$ value when all orbital is considered.

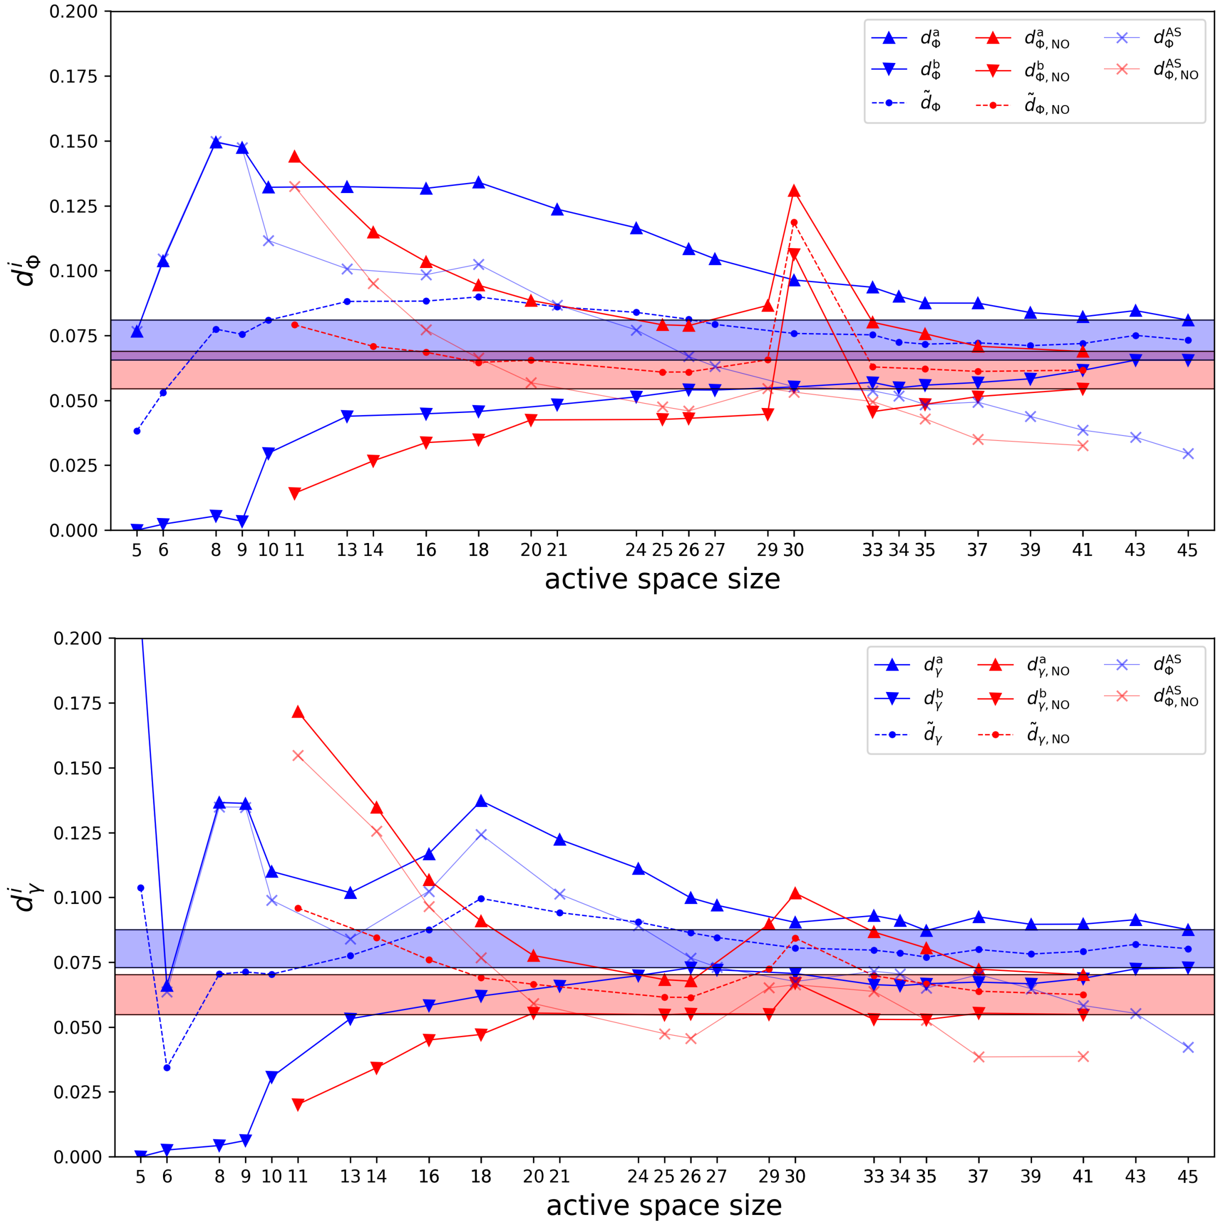


Figure S4: The dependence of $d^{\mathrm{a}}$, $d^{\mathrm{b}}$, and $\tilde{d}$ on active space size for $N_2O_4$. Upper figure is $d_\Phi$, lower figure is for $d_\gamma$ values, however $d$-s are determined for all active space selection procedure considered in this work. Upward triangles are for $d^{\mathrm{a}}$, downward triangles for $d^{\mathrm{b}}$, dots are for their average, $\tilde{d}$, and crosses are for $d^{\mathrm{AS}}$ values. Blue color represents canonical orbital selection, while red ones used natural orbitals The colored bands show the corresponding $d$ with the largest active space as a reference.

Here we can see, that after the local maximum in $d^{\mathrm{AS}}$ at 18 orbitals, the canonical $d^{\mathrm{a}}$ and $d^{\mathrm{b}}$ values are converging to the values from the largest active space with canonical

orbitals. The usage of $\tilde{d}$ is justified here, because its convergence is better than $d^{\mathrm{a}}$ and $d^{\mathrm{b}}$ for both $\Phi$ and $\gamma$. In case of natural orbitals, we can see a peak at 30 orbitals for every $d$-s. There is no obvious explanation for this. Possibly, the added orbital produces an unbalanced orbital set, which leads to a worse wavefunction composition, and has to be accompanied by other orbitals. This shows that there is room for improvement in this simple orbital selection procedure, for example, using mutual information. Besides that, the natural orbital transformation produces better active spaces again ($d^{\mathrm{AS}}_{\gamma,\mathrm{NO}} < d^{\mathrm{AS}}_{\gamma}$), and faster convergence, but $d^{\mathrm{a}}, d^{\mathrm{b}}$ and $\tilde{d}$ are converging to a different value as in the canonical case. This shows again the possible bias of using NO-s from a calculation with questionable reliability that leads to smaller $d$-s.

Obviously, we cannot perform such analysis in every case, and an appropriate threshold has to be determined for the determination of $\tilde{d}$. To this end, we will use two settings, a looser threshold of 0.1 and a tighter 0.05 for both $d^{\mathrm{AS}}_{\Phi}$ and $d^{\mathrm{AS}}_{\gamma}$. The corresponding results will be noted as $\tilde{d}_{\Phi}(0.1)$, $\tilde{d}_{\Phi}(0.05)$, $\tilde{d}_{\gamma}(0.1)$, $\tilde{d}_{\gamma}(0.05)$, where the number in the paranthesis is the used $d^{\mathrm{AS}}$ threshold. An additional restriction is that the active space selection error should be lower than with the previous active space candidate, to avoid a selection of active space before a local maximum.

# References


(1) Karton, A.; Sylvetsky, N.; Martin, J. M. L. W4-17: A diverse and high-confidence dataset of atomization energies for benchmarking high-level electronic structure methods. *J. Comput. Chem.* **2017**, *38*, 2063–2075.

(2) Xu, X.; Zhang, W.; Tang, M.; Truhlar, D. G. Do practical standard coupled cluster calculations agree better than Kohn–Sham calculations with currently available functionals when compared to the best available experimental data for dissociation energies of bonds to 3 d transition metals? *J. Chem. Theory Comput.* **2015**, *11*, 2036–2052.

Table S3: Pairwise Pearson correlation matrix of $\tilde{d}$ and other MR diagnostics for the W4-17 dataset. The more intense red hue represents higher correlation. The left and lower labels show the metrics, while the right and upper labels show the corresponding groups.

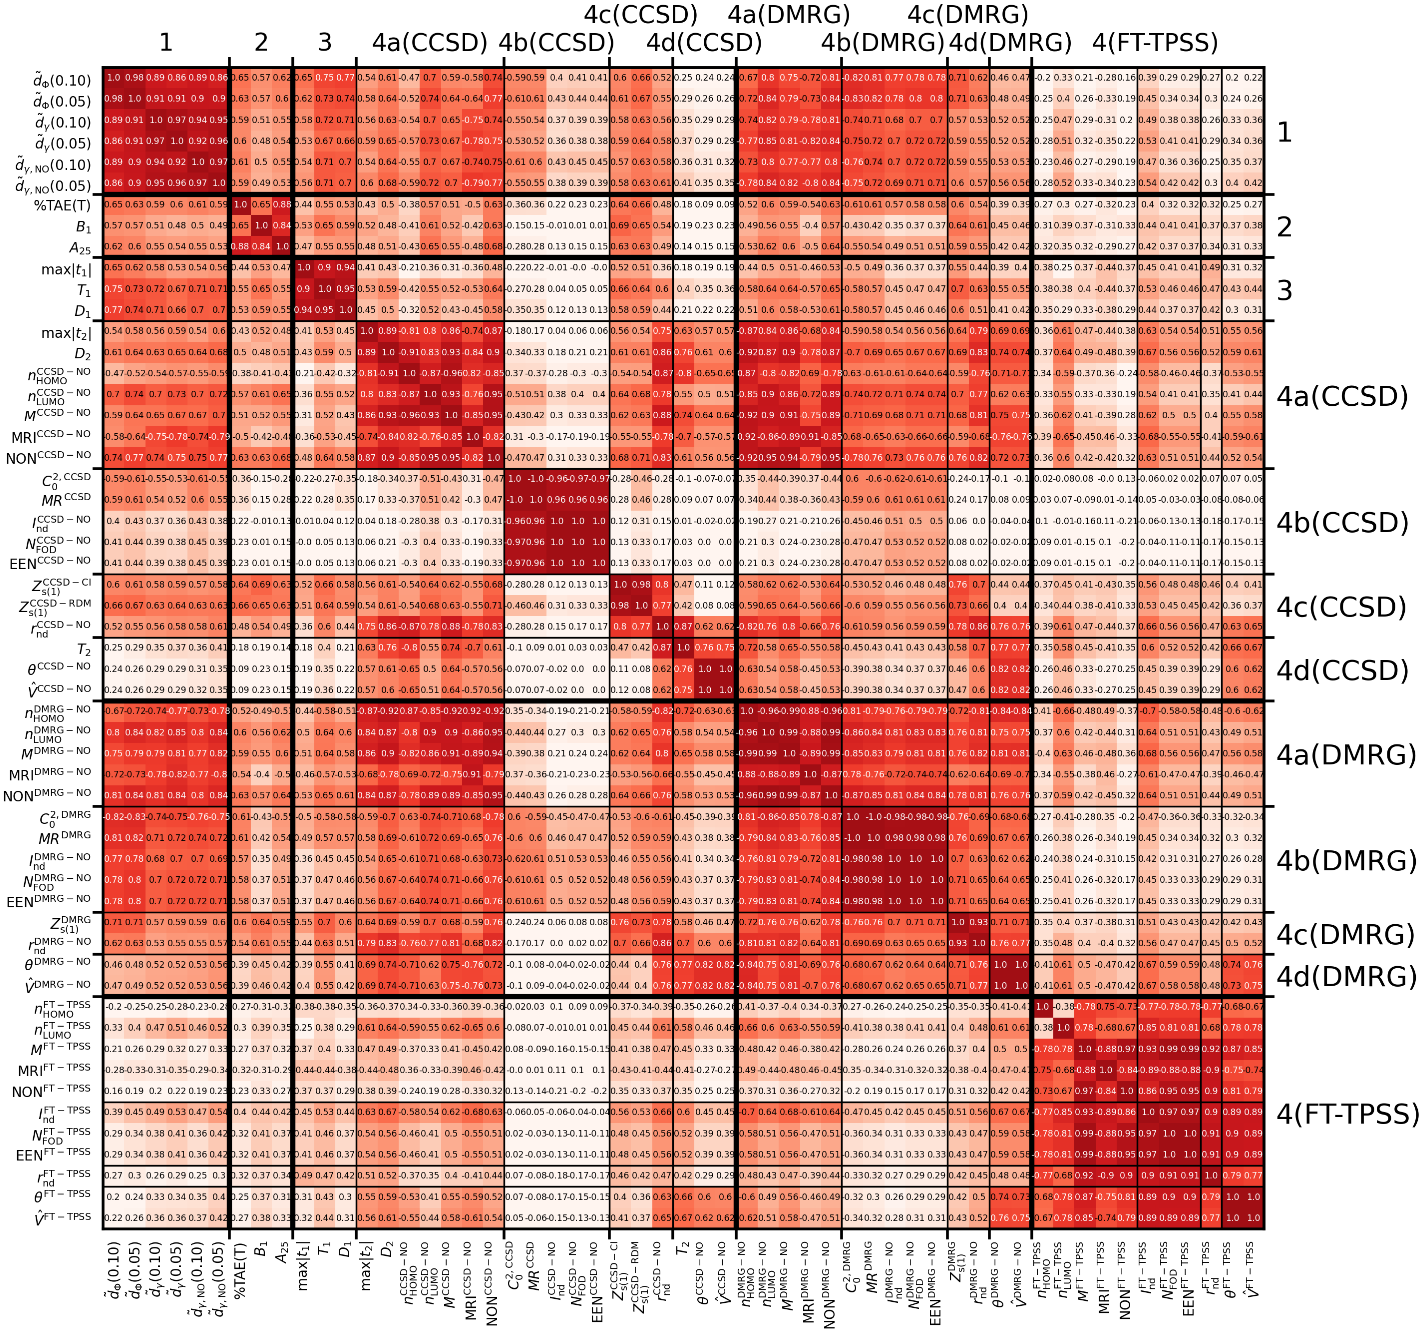

Table S4: Pairwise Kendall rank correlation matrix of $\tilde{d}$ and other MR diagnostics for the W4-17 dataset. The more intense red hue represents higher correlation. The left and lower labels show the metrics, while the right and upper labels show the corresponding groups.

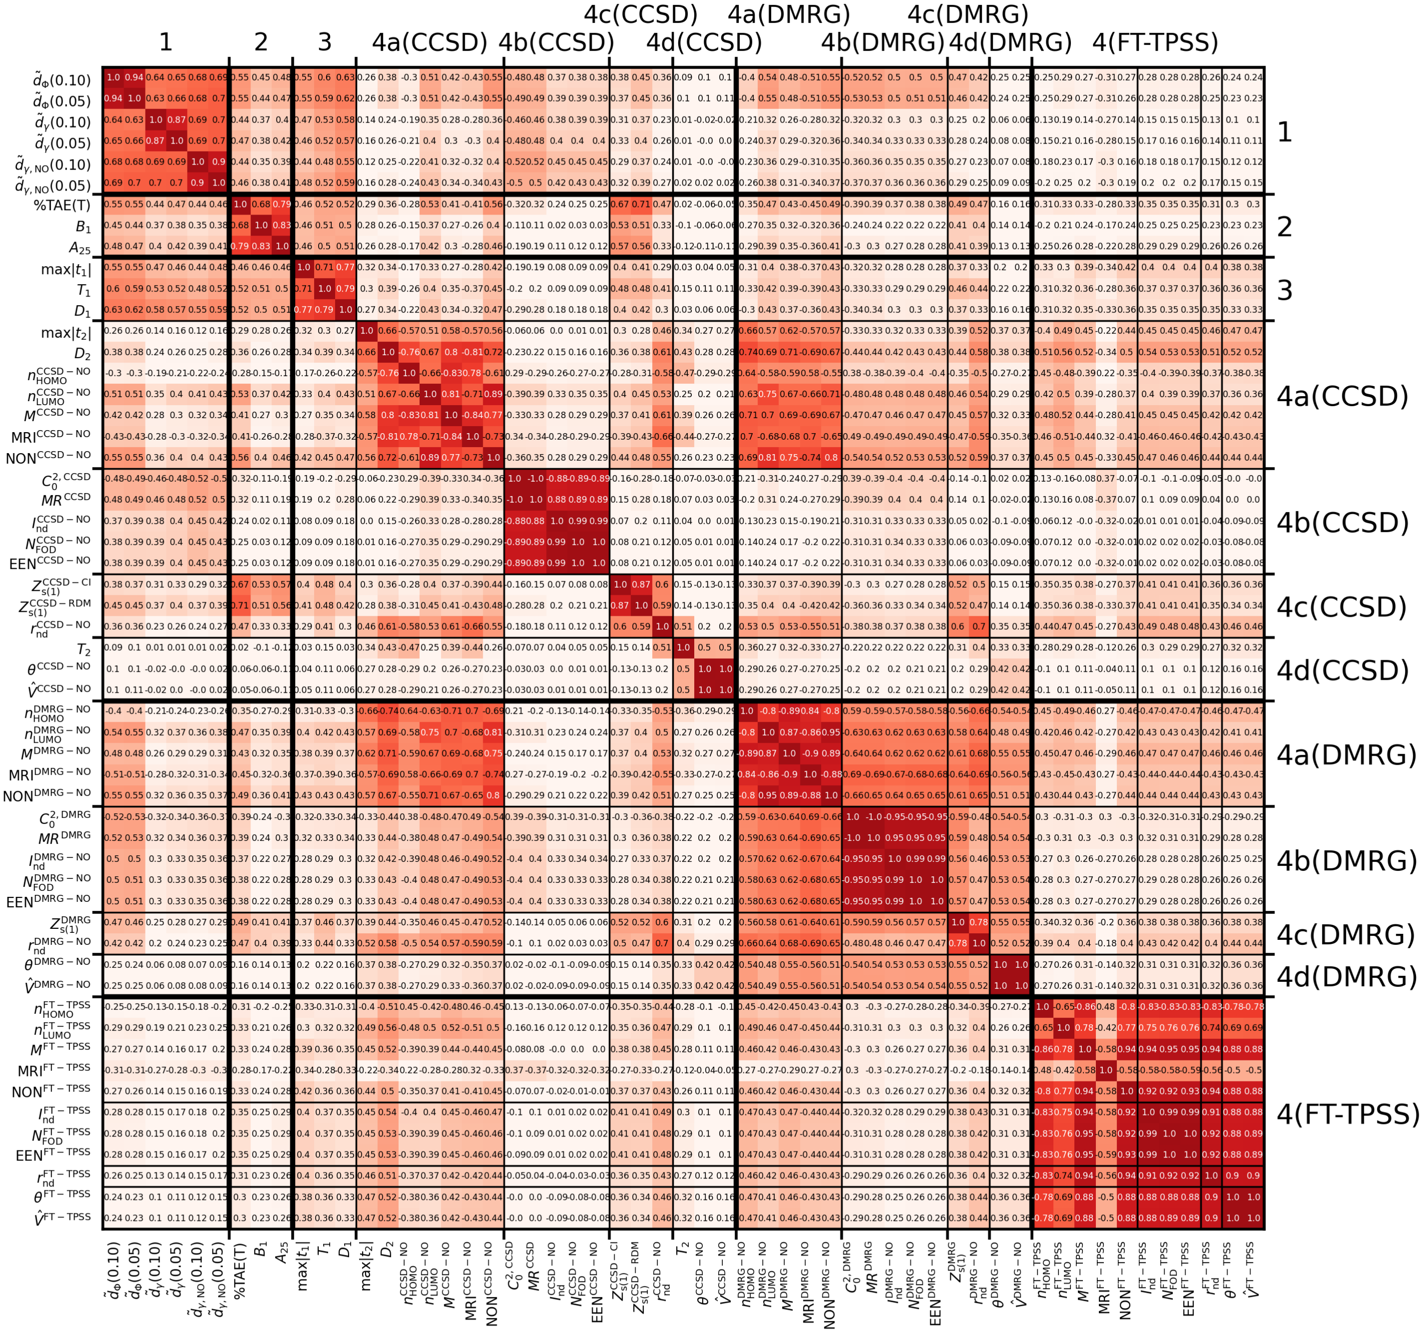

Table S5: Comparison of $\tilde{d} - s$ and their scaled version of alkanes and halogenated alkanes

| species | $\tilde{d}_\Phi(0.05)$ | $\tilde{d}_\gamma(0.05)$ | $\frac{\tilde{d}_\Phi(0.05)}{\sqrt{N_{\text{heavy}}}}$ | $\frac{\tilde{d}_\gamma(0.05)}{\sqrt{N_{\text{heavy}}}}$ |
|---|---|---|---|---|
| $CH_4$ | 0.013 | 0.013 | 0.013 | 0.013 |
| $CF_4$ | 0.027 | 0.028 | 0.012 | 0.013 |
| $CCl_4$ | 0.025 | 0.031 | 0.011 | 0.014 |
| $CHF_3$ | 0.025 | 0.029 | 0.013 | 0.014 |
| $CH_3F$ | 0.017 | 0.021 | 0.012 | 0.015 |
| $CH_2F_2$ | 0.019 | 0.024 | 0.011 | 0.014 |
| $CH_2ClF$ | 0.021 | 0.026 | 0.012 | 0.015 |
| $CF_2Cl_2$ | 0.018 | 0.036 | 0.008 | 0.016 |
| $CCl_3H$ | 0.020 | 0.028 | 0.010 | 0.014 |
| $CClH_3$ | 0.013 | 0.020 | 0.009 | 0.014 |
| $C_2H_6$ | 0.011 | 0.017 | 0.008 | 0.012 |
| $C_2F_6$ | 0.041 | 0.045 | 0.014 | 0.016 |
| $C_2Cl_6$ | 0.012 | 0.043 | 0.004 | 0.015 |
| $C_2H_5F$ | 0.021 | 0.023 | 0.012 | 0.013 |
| $C_2ClH_5$ | 0.023 | 0.025 | 0.013 | 0.014 |
| $C_3H_8$ | 0.024 | 0.021 | 0.014 | 0.012 |
| $C_4H_{10}$ | 0.023 | 0.022 | 0.012 | 0.011 |
| $C_5H_{12}$ | 0.024 | 0.023 | 0.011 | 0.010 |


(3) Welch, B. K.; Almeida, N. M. S.; Wilson, A. K. Super ccCA (s-ccCA): an approach for accurate transition metal thermochemistry. *Mol. Phys.* **2021**, *119*, e1963001.

(4) Jiang, W.; DeYonker, N. J.; Wilson, A. K. Multireference character for 3d transition-metal-containing molecules. *J. Chem. Theory Comput.* **2012**, *8*, 460–468.

(5) Wang, J.; Manivasagam, S.; Wilson, A. K. Multireference character for 4d transition metal-containing molecules. *J. Chem. Theory Comput.* **2015**, *11*, 5865–5872.

(6) Süß, D.; Huber, S. E.; Mauracher, A. On the impact of multi-reference character of small transition metal compounds on their bond dissociation energies. *J. Chem. Phys.* **2020**, *152*.
